# Supplementary material for: Bond-breaking Induced Lifshitz Transition in Robust Dirac Semimetal $\mathbf{VAl_3}$
Source: arXiv:2005.07970 source file (2020-05-16)
Supplement: Supplementary file 1 [file Arxiv_VAl_SI.pdf]

# Supplementary Information for Bond-breaking Induced Lifshitz Transition in Robust Dirac Semimetal $VAl_3$

Yiyuan Liu⋆,[1] Yu-Fei Liu,[1] Xin Gui,[2] Cheng Xiang,[1] Hui-bin Zhou,[1] Chuang-Han Hsu,[3,4] Hsin Lin,[5] Tay-Rong Chang,[6,7,8] Weiwei Xie,[2] and Shuang Jia[1,9,10,11,*]

[1]*International Center for Quantum Materials, School of Physics, Peking University, China*

[2]*Department of Chemistry, Louisiana State University, Baton Rouge, LA 70803, USA*

[3]*Departments of Physics, National University of Singapore, Singapore 117542*

[4]*Centre for Advanced 2D Materials and Graphene Research Centre, National University of Singapore, Singapore 117546*

[5]*Institute of Physics, Academia Sinica, Taipei 11529, Taiwan*

[6]*Department of Physics, National Cheng Kung University, Tainan 701, Taiwan*

[7]*Center for Quantum Frontiers of Research & Technology (QFort), Tainan 701, Taiwan*

[8]*Physics Division, National Center for Theoretical Sciences, Hsinchu, Taiwan*

[9]*Collaborative Innovation Center of Quantum Matter, Beijing 100871, China*

[10]*CAS Center for Excellence in Topological Quantum Computation, University of Chinese Academy of Science, Beijing 100190, China*

[11]*Beijing Academy of Quantum Information Sciences, West Building 3, No. 10 Xibeiwang East Road, Haidian District, Beijing 100193,China*

PACS numbers:

[*]Electronic address: gwljiashuang@pku.edu.cn

## Supplementary text

### Crystal Structure of $TAl_3$

The trialuminide compounds with early transition metals (T = Sc, Ti, Zr, V, Nb, Ta) crystallize in three closely related $AuCu_3$-, $ZrAl_3$- and $TiAl_3$-type structures [1–5]. All three structures are built from the $Al_{12}$ cuboctehedra containing T atoms with different arrangements of the $TAl_{12}$ units (Fig.S1) [6, 7]. These cuboctehra are arranged in a primitive cubic fashion through shared square faces in $ScAl_3$. In $TiAl_3$-type structure, each layer of T atoms is shifted by $(1/2, 1/2, 0)$ leading to a doubling of the unit cell. In $ZrAl_3$-type structure the shifts occur every two T atom layers. This series of aluminides owns this trend: with the increase of electrons, the crystal cells grow to be more flat by the change of atomic environment. This trend is obvious if we compare the nearest T neighbors of the T atoms: there are six scandium atoms nearest to scandium atom, five to zirconium atom, and only four to vanadium atom forming a planar T net.

### Temperature-dependent resistivity for $V_{1-x}Ti_xAl_3$

Figure S2 shows the normalized temperature-dependent resistivity ($\rho/\rho_{300K}$) for $V_{1-x}Ti_xAl_3$. While all the samples show metallic $\rho$(T), we notice that the profile for $x \leq 0.35$ is different from that for $x > 0.35$. When $x$ is larger than 0.35, the $\rho$(T) increases linearly with increasing temperature above 100 K and $d\rho/d$T is nearly invariant from 100 K to 300 K (Fig.S1 c and d). This linear temperature-dependent $\rho$(T) fits the phonon scattering of the electrons in metal. When $x$ is less than 0.35, the $\rho$(T) curves deviate from linear dependence in high temperature while $d\rho/d$T shows a hump around 50 K to 150 K. The nonlinear $\rho$(T) is likely due to the carrier density change in semimetal with increasing temperature (See Fig. 3 in the main text).

### Stronger interlayer interaction in $VAl_3$

Figure S3 illustrates the highest occupied molecular orbitals (HOMOs) and lowest unoccupied molecular orbitals (LUMOs) for $TiAl_3$, $NbAl_3$ and $VAl_3$. Although $VAl_3$ and $NbAl_3$ own the same number of electrons, the electron cloud in $VAl_3$ distributing near the inter-

layer V-Al bond is denser than that in $TiAl_3$ and $NbAl_3$. $VAl_3$ owns shorter bond length and stronger native interaction.

**Lattice parameters for $V_{1-x}Ti_xAl_3$**

Figure S4 shows the lattice parameters of $TAl_3$ (T = Ti, V, Nb and Ta) and representative samples in $V_{1-x}Ti_xAl_3$ solid solutions.The unit cells (UCs) of $TiAl_3$, $NbAl_3$ and $TaAl_3$ have similar size while the UC of $VAl_3$ is 8% smaller in volume. The small UC of $VAl_3$ is due to its strong chemical bonds. It is noteworthy that the lattice parameters of $V_{1-x}Ti_xAl_3$ change in a larger pace for $0 < x < 0.4$ than that for $0.4 < x < 1$. The anomalous structure distortion for $0.3 < x < 0.4$ is apparent in Fig. 4 of the main text.

***n*-*p* transition in thermoelectricity**

In order to verify the *n*-*p* transition in $V_{1-x}Ti_xAl_3$, we measured the Seebeck coefficient (S) from 100 K to 300 K for selected samples (Fig. S5). Consistent with the Hall measurements, there also exists a sign change of S from $x = 0.05$ to 0.1 in the series. Since the sign of S for semimetals is determined by complicated factors such as scattering rate and populations of electron and hole, the sign reversal point is different from the Hall signal. The S value for $VAl_3$ ($\sim 50\mu V/K$) is close to the theoretic limit of metal [8], indicating a semimetal state. In contrast the S value for $TiAl_3$ ($6.7\mu V/K$) is as small as that expected for the metal with high carrier density like Cu ($1.3\mu V/K$).

**Magnetic properties of single-crystalline $VAl_3$**

Temperature-dependent molar susceptibility of $VAl_3$ is measured under 1 kOe magnetic field along the crystallographic *c* axis as shown in Fig. S6. Field-dependent magnetization of $VAl_3$ at 2 K is presented in Fig. S7. The temperature-dependent magnetization is diamagnetic with a Curie tail below 50 K which is likely coming from a small amount of paramagnetic impurity. The paramagnetic impurity can be identified in the M(H) curve under low field at 2 K. The kink at 30 kOe in the M(H) curve is likely coming from the low-frequency dHvA quantum oscillations.

**Single crystal X-ray diffraction data**

Table S1, S2 and S3 lists the single crystal X-ray diffraction data for $V_{1-x}Ti_xAl_3$ ($x = 0$, 0.2, 0.4, 0.6, 0.8 and 1). All the samples crystallize in tetragonal $TiAl_3$-type structure. Please note because the X-ray diffraction cannot distinguish V and Al atoms, the refined occupancy of V and Ti is largely deviated from the EDS results. The single crystal XRD result is consistent with the powder X-ray diffraction and verifies that $V_{1-x}Ti_xAl_3$ are isostructural solid solutions.

---


[1] Freeman AJ, Hong T, Lin W and Xu Jian-Hua, Phase Stability and Role of Ternary Additions on Electronic and Mechanical Properties of Aluminum Intermetallics *MRS Online Proceedings Library Archive*, 213 (1990)

[2] Xu Jian-hua and Freeman Arthur J, Band filling and structural stability of cubic trialuminides: $YAl_3$, $ZrAl_3$, and $NbAl_3$ *Physical Review B*, 40, 11927 (1989)

[3] Hong T, Watson-Yang TJ, Freeman Arthur J, Oguchi T and Xu Jian-hua, Crystal structure, phase stability, and electronic structure of Ti-Al intermetallics: $TiAl_3$ *Physical Review B*, 41, 12462 (1990)

[4] Xu J-H and Freeman Arthur J, Phase stability and electronic structure of $ScAl_3$ and $ZrAl_3$ and of Sc-stabilized cubic $ZrAl_3$ precipitates *Physical Review B*, 41, 12553 (1990)

[5] Vajenine Grigori V and Hoffmann Roald, Magic electron counts for networks of condensed clusters: Vertex-sharing aluminum octahedra *Journal of the American Chemical Society*, 120, 4200 (1998)

[6] Kilduff Brandon J, Yannello Vincent J, Fredrickson Daniel C, Defusing Complexity in Intermetallics: How Covalently Shared Electron Pairs Stabilize the FCC Variant $Mo_2Cu_xGa_{6-x}$($x \approx 0.9$) *Inorganic chemistry*, 54, 8103 (2015)

[7] Yannello Vincent J and Fredrickson Daniel C, Generality of the 18-n rule: intermetallic structural chemistry explained through isolobal analogies to transition metal complexes *Inorganic chemistry*, 54, 11385 (2015)

[8] Behnia Kamran, *Fundamentals of thermoelectricity*, OUP Oxford Press (2015)

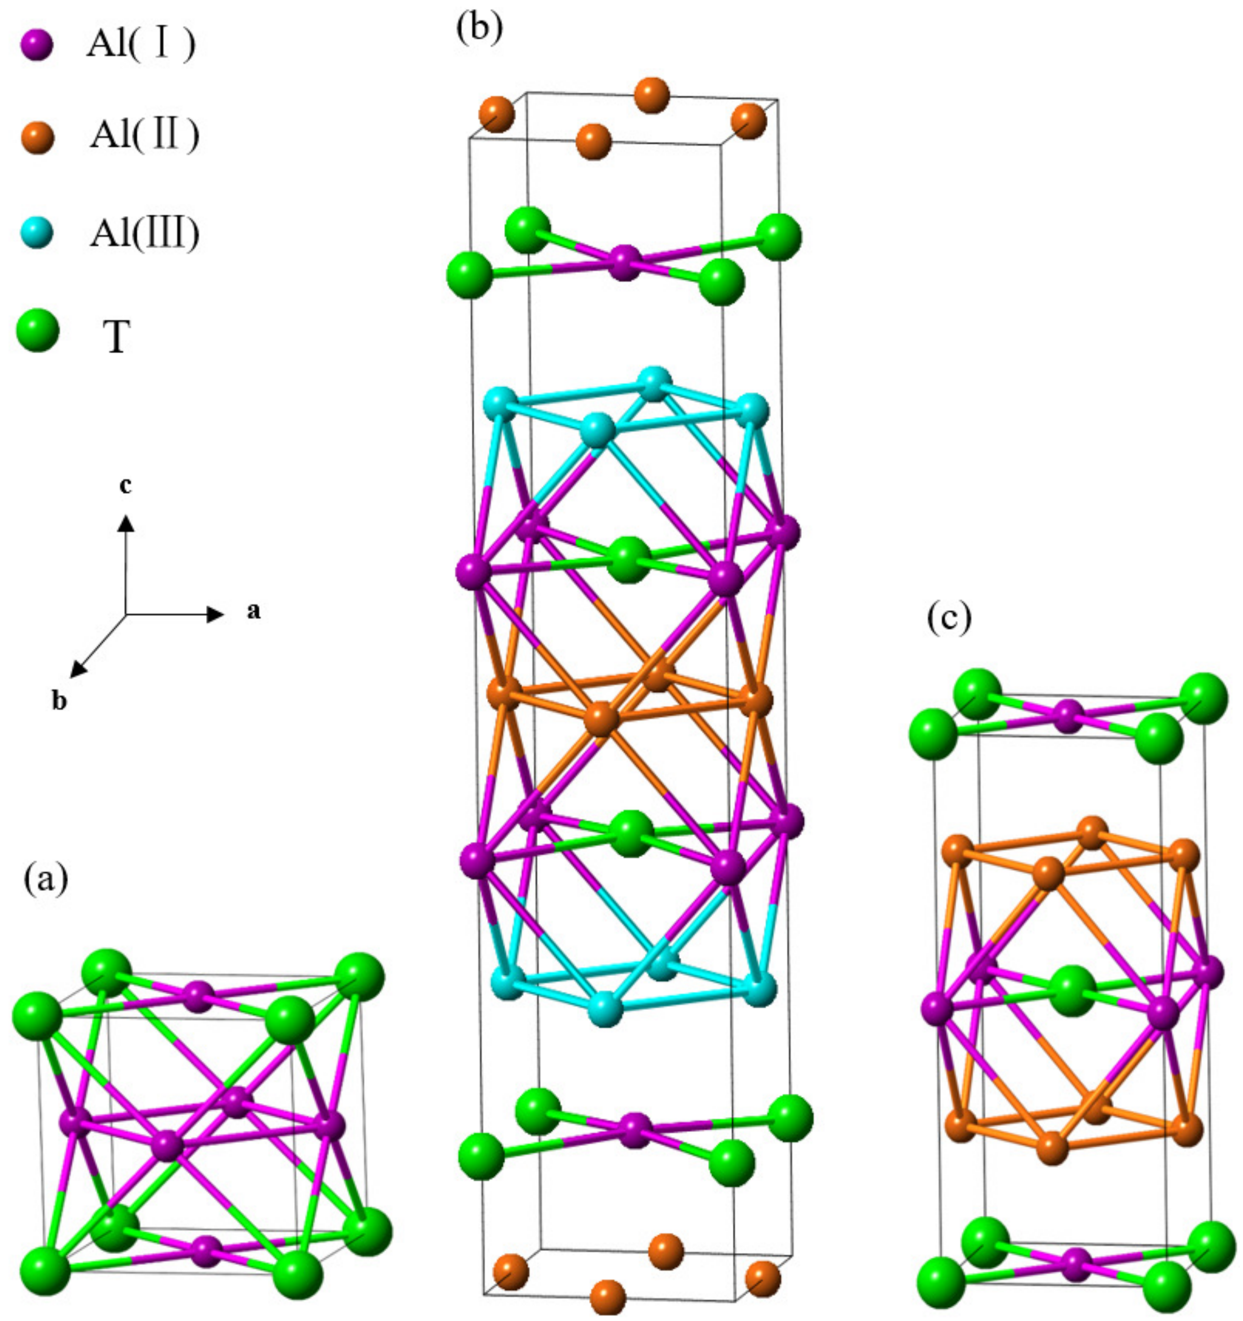


FIG. 1: Crystal structures of $TAl_3$. (A): $ScAl_3$, $AuCu_3$-type, (B): $ZrAl_3$, $ZrAl_3$-type ; (C): $TiAl_3$, $TiAl_3$-type.

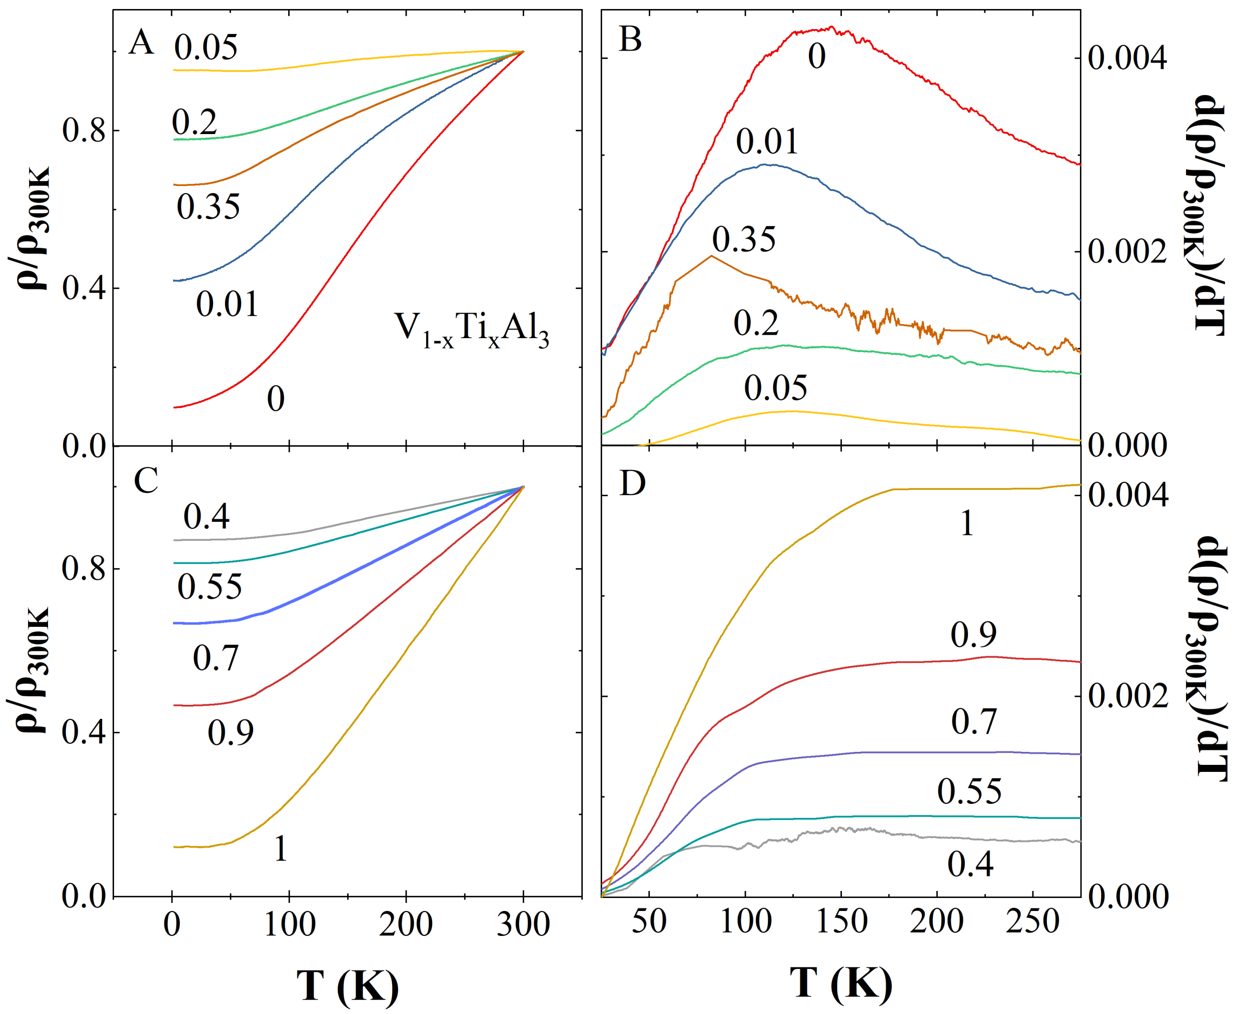


FIG. 2: Temperature-dependent resistivity (presented as $\rho/\rho_{300\mathrm{K}}$) and $d(\rho/\rho_{300\mathrm{K}})/d\mathrm{T}$ for $\mathrm{V}_{1-x}\mathrm{Ti}_x\mathrm{Al}_3$. (A) and (B): The representative samples for $0 \leq x \leq 0.35$; (C) and (D): For $0.35 < x \leq 1$

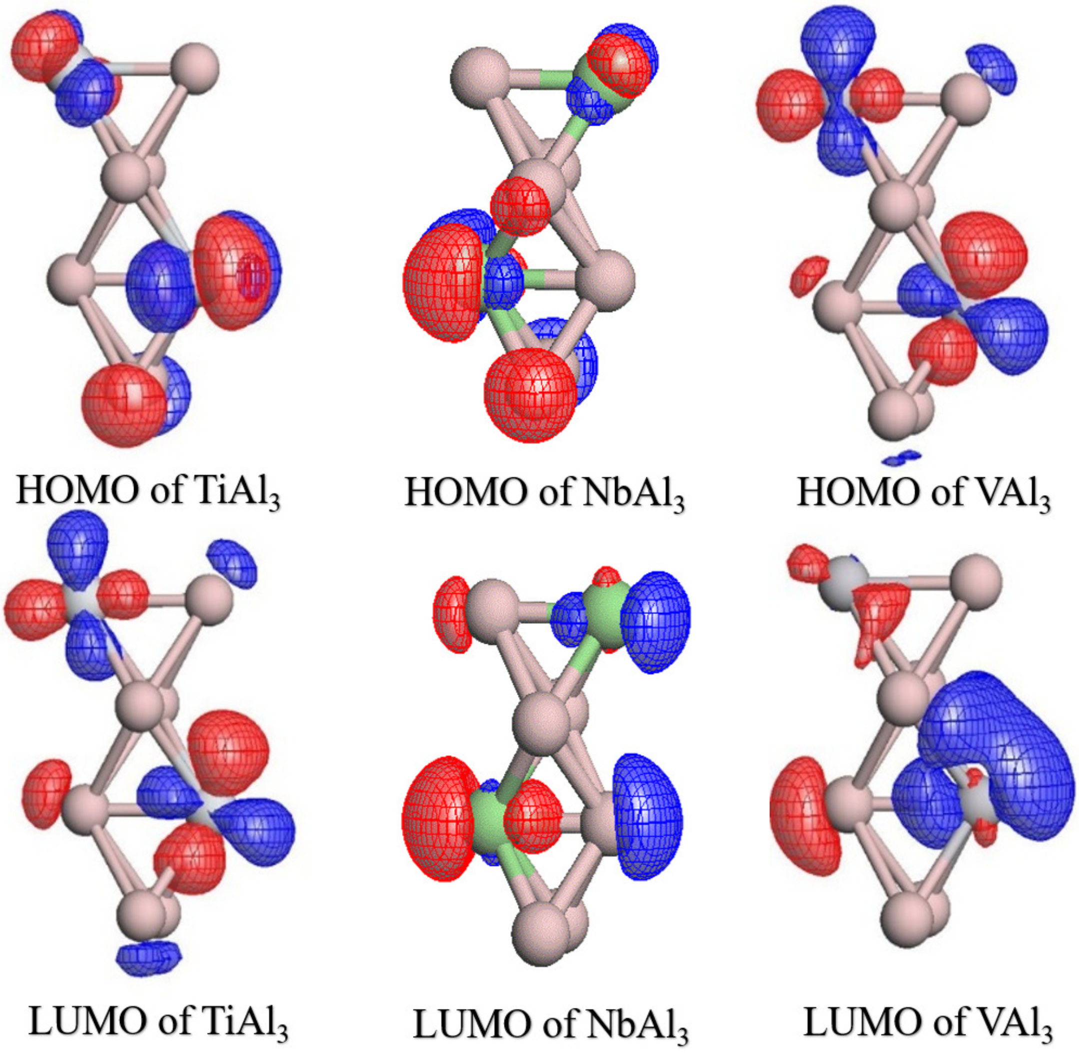


FIG. 3: HOMO and LUMO of $TiAl_3$, $NbAl_3$ and $VAl_3$.

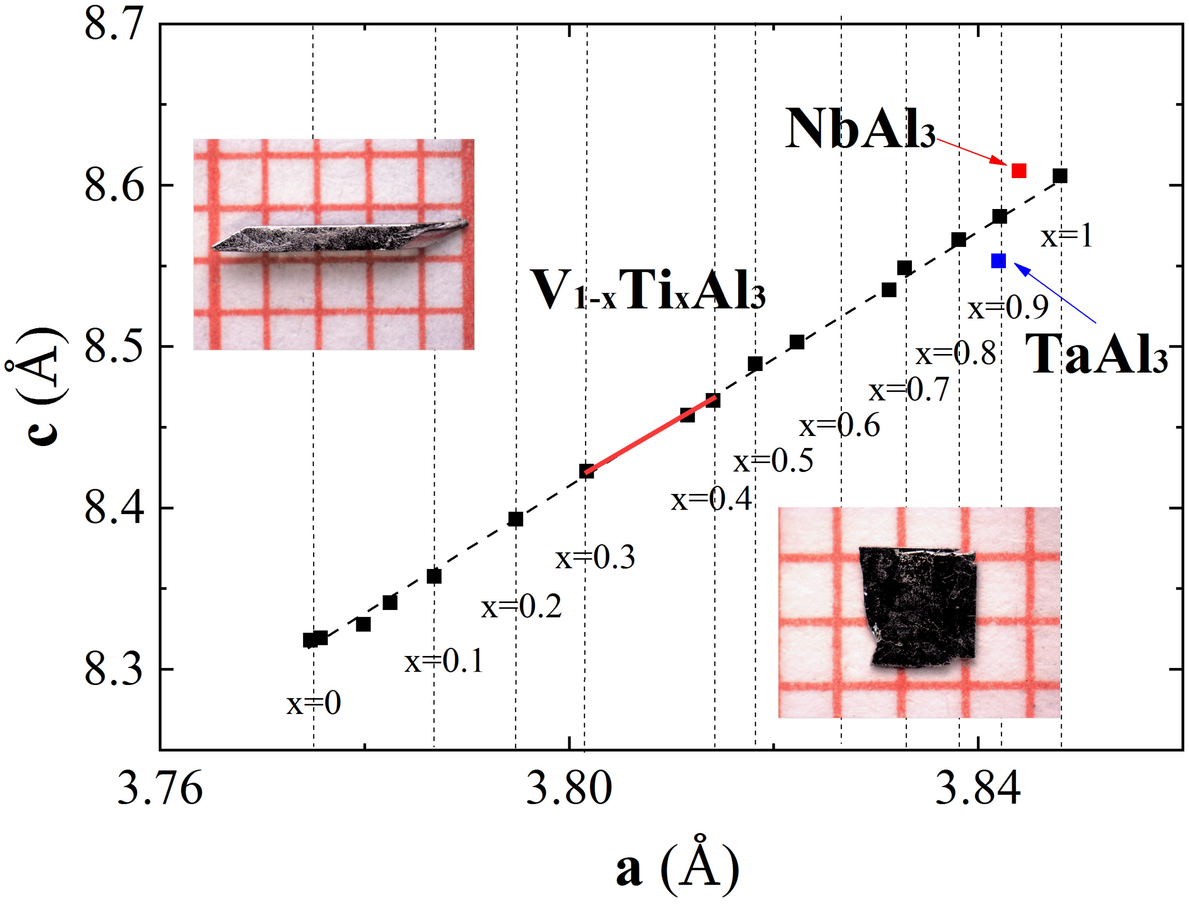


FIG. 4: Lattice parameters of $V_{1-x}Ti_xAl_3$. The straight dashed line is guided by eye. The dotted lines demonstrate the positions of $a$ and $c$ for x changing every 0.1. Insets: photos of $VAl_3$ (upper-left) and $TiAl_3$ (down-right). The lattice parameters of $NbAl_3$ and $TaAl_3$ are presented in the diagram as comparison.

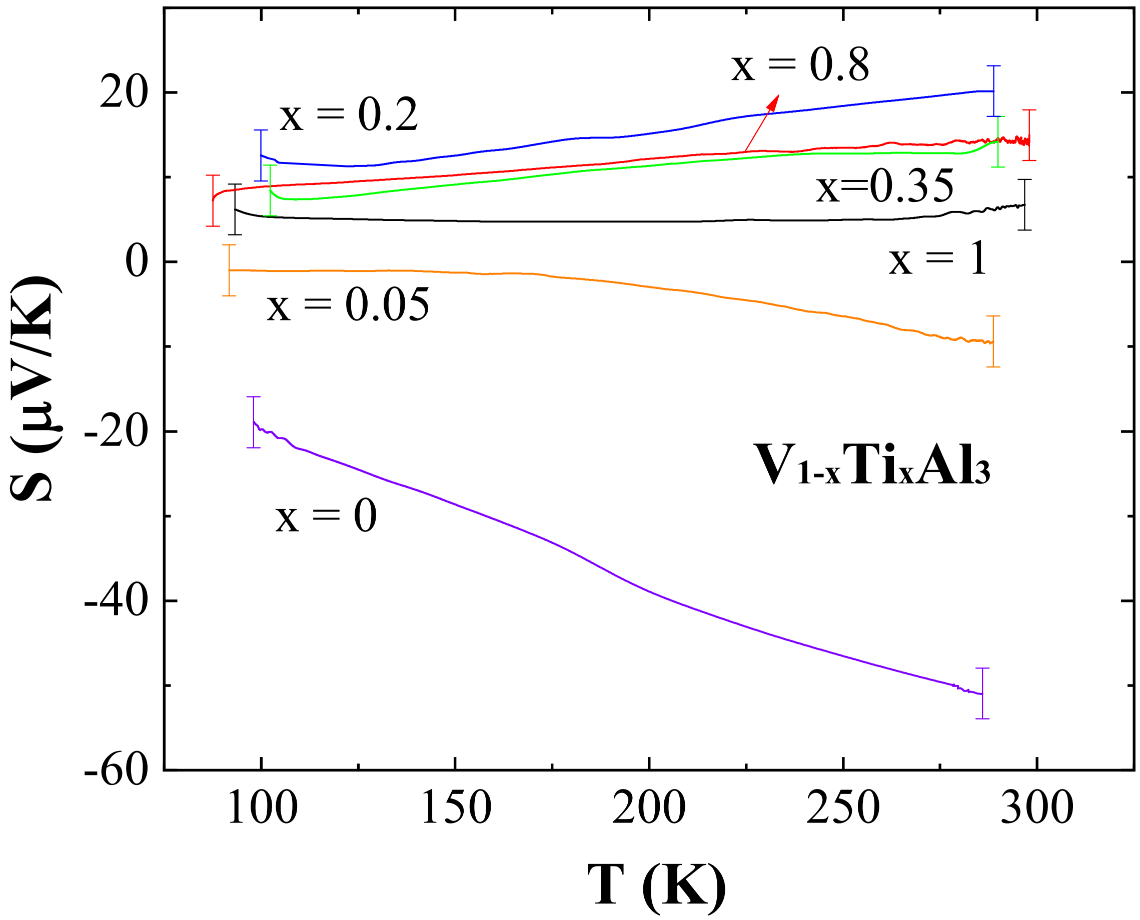


FIG. 5: Seebeck coefficients for the representative samples in $V_{1-x}Ti_xAl_3$ from 100 K to room temperature. The error bar is estimated as $\pm 4$ $\mu$V/K.

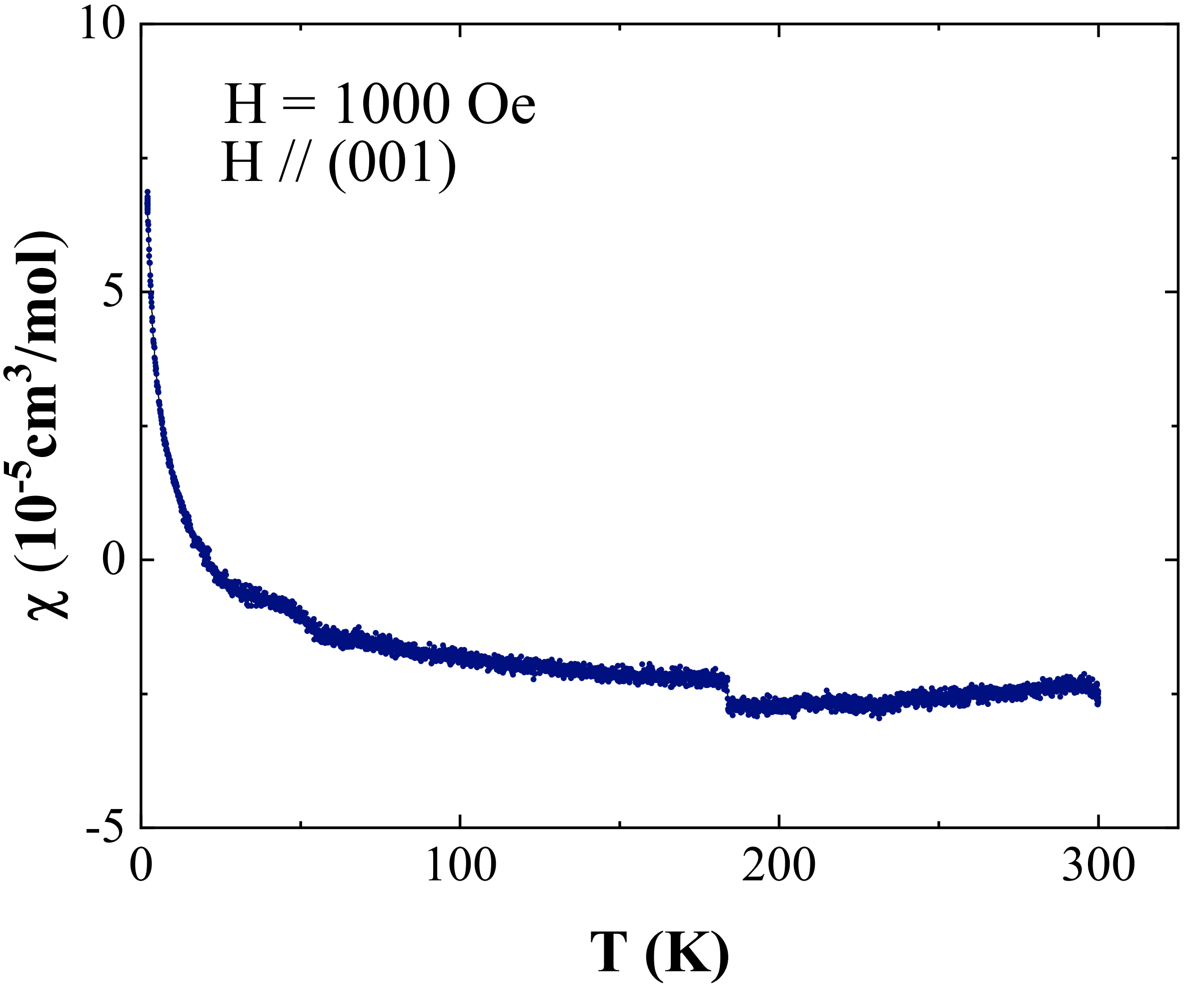


FIG. 6: Temperature-dependent molar susceptibility of $VAl_3$

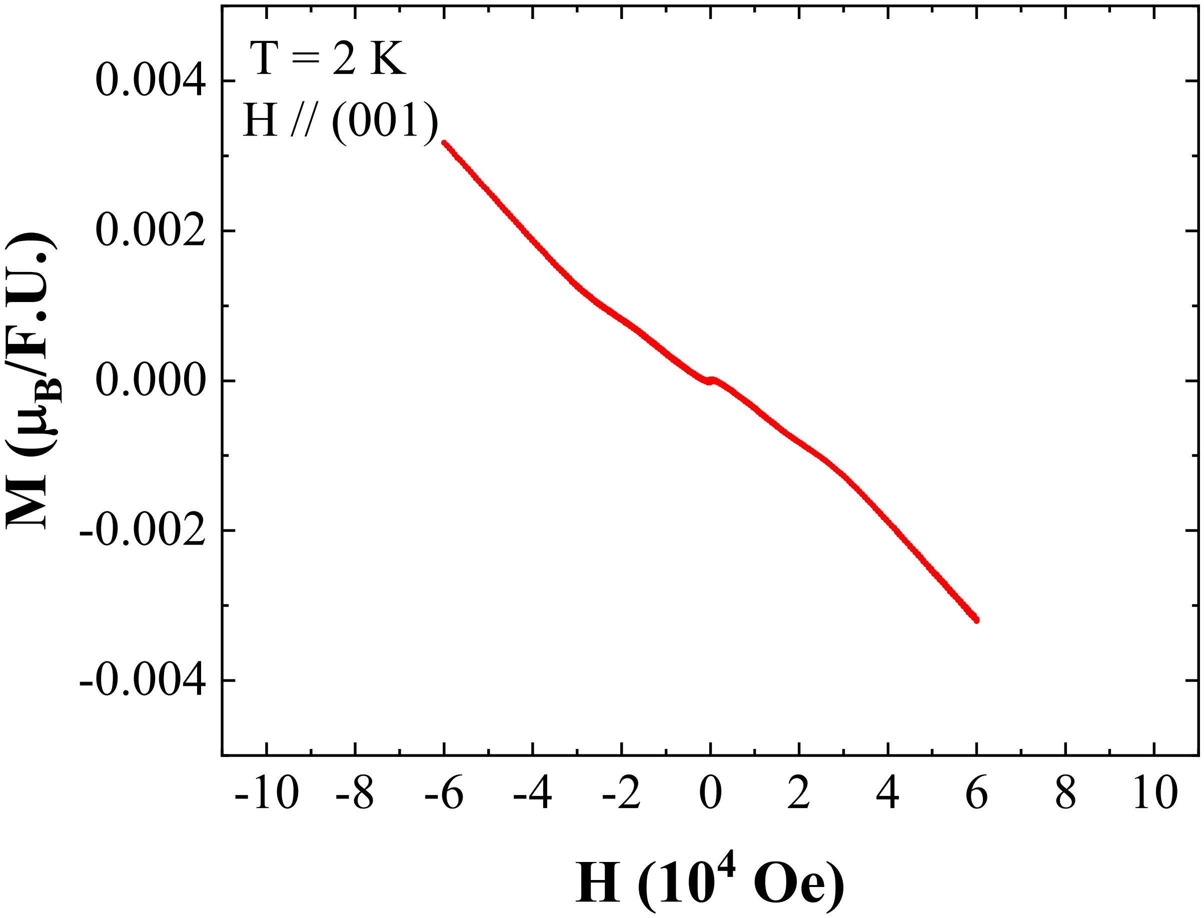


FIG. 7: Field-dependent magnetization of $VAl_3$ at 2 K

TABLE I: Single crystal XRD refinement for $V_{1-x}Ti_xAl_3$ system at 296(2) K.

| Label | $TiAl_3$ | $V_{0.2}Ti_{0.8}Al_3$ | $V_{0.4}Ti_{0.6}Al_3$ | $V_{0.6}Ti_{0.4}Al_3$ | $V_{0.8}Ti_{0.2}Al_3$ | $VAl_3$ |
|---|---|---|---|---|---|---|
| Refined Formula | $TiAl_3$ | $V_{0.03(8)}Ti_{0.97(8)}Al_3$ | $V_{0.12(10)}Ti_{0.88(10)}Al_3$ | $V_{0.56(6)}Ti_{0.44(6)}Al_3$ | $V_{0.71(5)}Ti_{0.29(5)}Al_3$ | $VAl_3$ |
| F.W. (g/mol) | 128.84 | 128.93 | 129.22 | 130.54 | 130.98 | 131.88 |
| Space group; Z | I 4/mmm; 2 | I 4/mmm; 2 | I 4/mmm; 2 | I 4/mmm; 2 | I 4/mmm; 2 | I 4/mmm; 2 |
| a(Å) | 3.851 (3) | 3.841 (1) | 3.834 (1) | 3.811 (1) | 3.795 (1) | 3.783(1) |
| c(Å) | 8.621 (6) | 8.576 (2) | 8.560 (2) | 8.464 (2) | 8.398 (2) | 8.333(3) |
| V (Å$^3$) | 127.8 (2) | 126.50 (7) | 125.8 (1) | 122.95 (5) | 120.94 (5) | 119.3 |
| Extinction Coefficient | 0.26 (1) | 0.32 (3) | 0.11 (2) | 0.07 (1) | 0.008 (3) | 0.002(3) |
| $\theta$ range (deg) | 4.729 - 32.983 | 4.754 - 33.181 | 4.763 - 33.204 | 4.817 - 32.972 | 4.855 - 33.152 | 4.893 - 33.043 |
| No. reflections; $R_{int}$ | 657; 0.0335 | 616; 0.0199 | 656; 0.0174 | 743; 0.0214 | 813; 0.0151 | 612; 0.0194 |
| No. independent reflections | 95 | 95 | 95 | 91 | 91 | 88 |
| No. parameters | 8 | 9 | 9 | 9 | 9 | 8 |
| $R_1$: $R_2$ (I¿2$\delta$(I)) | 0.0157; 0.0259 | 0.0090; 0.0207 | 0.0134; 0.0300 | 0.0063; 0.0171 | 0.0070; 0.0153 | 0.0114; 0.0269 |
| Goodness of fit | 1.141 | 1.282 | 1.424 | 1.286 | 1.124 | 1.113 |
| Diffraction peak and hole ($e^-$/ Å$^3$) | 0.536; -0.247 | 0.226; -0.372 | 0.261; -0.535 | 0.126; -0.132 | 0.167; -0.185 | 0.242; -0.335 |

TABLE II: Atomic coordinates and equivalent isotropic displacement parameters of $V_{1-x}Ti_xAl_3$ system. ($U_{eq}$ is defined as one-third of the trace of the orthogonalized $U_{ij}$ tensor (Å$^2$))

$TiAl_3$

| Atom | Wyck. | Occ. | x | y | z | $U_{eq}$ |
|---|---|---|---|---|---|---|
| Ti1 | 2a | 1 | 0 | 0 | 0 | 0.0043 (2) |
| Al2 | 4d | 1 | 1/2 | 0 | 1/4 | 0.0068 (2) |
| Al3 | 2b | 1 | 0 | 0 | 1/2 | 0.0074 (2) |

$V_{0.2}Ti_{0.8}Al_3$

| Atom | Wyck. | Occ. | x | y | z | $U_{eq}$ |
|---|---|---|---|---|---|---|
| V1 | 2a | 0.03 (8) | 0 | 0 | 0 | 0.0050 (3) |
| Ti2 | 2a | 0.97 (8) | 0 | 0 | 0 | 0.0050 (3) |
| Al3 | 4d | 1 | 1/2 | 0 | 1/4 | 0.0069 (3) |
| Al4 | 2b | 1 | 0 | 0 | 1/2 | 0.0075 (3) |

$V_{0.4}Ti_{0.6}Al_3$

| Atom | Wyck. | Occ. | x | y | z | $U_{eq}$ |
|---|---|---|---|---|---|---|
| V1 | 2a | 0.12 (10) | 0 | 0 | 0 | 0.0049 (3) |
| Ti2 | 2a | 0.88 (10) | 0 | 0 | 0 | 0.0049 (3) |
| Al3 | 4d | 1 | 1/2 | 0 | 1/4 | 0.0069 (4) |
| Al4 | 2b | 1 | 0 | 0 | 1/2 | 0.0076 (4) |

$V_{0.6}Ti_{0.4}Al_3$

| Atom | Wyck. | Occ. | x | y | z | $U_{eq}$ |
|---|---|---|---|---|---|---|
| V1 | 2a | 0.56 (6) | 0 | 0 | 0 | 0.0045 (2) |
| Ti2 | 2a | 0.44 (6) | 0 | 0 | 0 | 0.0045 (2) |
| Al3 | 4d | 1 | 1/2 | 0 | 1/4 | 0.0062 (3) |
| Al4 | 2b | 1 | 0 | 0 | 1/2 | 0.0068 (3) |

$V_{0.8}Ti_{0.2}Al_3$

| Atom | Wyck. | Occ. | x | y | z | $U_{eq}$ |
|---|---|---|---|---|---|---|
| V1 | 2a | 0.71 (5) | 0 | 0 | 0 | 0.0048 (1) |
| Ti2 | 2a | 0.29 (5) | 0 | 0 | 0 | 0.0048 (1) |
| Al3 | 4d | 1 | 1/2 | 0 | 1/4 | 0.0069 (2) |
| Al4 | 2b | 1 | 0 | 0 | 1/2 | 0.0075 (2) |

$VAl_3$

| Atom | Wyck. | Occ. | x | y | z | $U_{eq}$ |
|---|---|---|---|---|---|---|
| V1 | 2a | 1 | 0 | 0 | 0 | 0.0048 (2) |
| Al2 | 4d | 1 | 1/2 | 0 | 1/4 | 0.0066 (2) |
| Al3 | 2b | 1 | 0 | 0 | 1/2 | 0.0070 (2) |

TABLE III: Anisotropic thermal displacements from $V_{1-x}Ti_xAl_3$ system.

$TiAl_3$

| Atom | U11 | U22 | U33 | U23 | U13 | U12 |
|---|---|---|---|---|---|---|
| Ti1 | 0.0048 (2) | 0.0048 (2) | 0.0033 (3) | 0 | 0 | 0 |
| Al2 | 0.0073 (2) | 0.0073 (2) | 0.0058 (3) | 0 | 0 | 0 |
| Al3 | 0.0063 (3) | 0.0063 (3) | 0.0094 (4) | 0 | 0 | 0 |

$V_{0.2}Ti_{0.8}Al_3$

| Atom | U11 | U22 | U33 | U23 | U13 | U12 |
|---|---|---|---|---|---|---|
| V1 | 0.0054 (3) | 0.0054 (3) | 0.0043 (3) | 0 | 0 | 0 |
| Ti2 | 0.0054 (3) | 0.0054 (3) | 0.0043 (3) | 0 | 0 | 0 |
| Al3 | 0.0071 (3) | 0.0071 (3) | 0.0063 (4) | 0 | 0 | 0 |
| Al4 | 0.0065 (4) | 0.0065 (4) | 0.0094 (4) | 0 | 0 | 0 |

$V_{0.4}Ti_{0.6}Al_3$

| Atom | U11 | U22 | U33 | U23 | U13 | U12 |
|---|---|---|---|---|---|---|
| V1 | 0.0051 (3) | 0.0051 (3) | 0.0046 (3) | 0 | 0 | 0 |
| Ti2 | 0.0051 (3) | 0.0051 (3) | 0.0046 (3) | 0 | 0 | 0 |
| Al3 | 0.0071 (4) | 0.0071 (4) | 0.0063 (5) | 0 | 0 | 0 |
| Al4 | 0.0068 (4) | 0.0068 (4) | 0.0093 (5) | 0 | 0 | 0 |

$V_{0.6}Ti_{0.4}Al_3$

| Atom | U11 | U22 | U33 | U23 | U13 | U12 |
|---|---|---|---|---|---|---|
| V1 | 0.0044 (2) | 0.0044 (2) | 0.0047 (2) | 0 | 0 | 0 |
| Ti2 | 0.0044 (2) | 0.0044 (2) | 0.0047 (2) | 0 | 0 | 0 |
| Al3 | 0.0060 (3) | 0.0060 (3) | 0.0066 (3) | 0 | 0 | 0 |
| Al4 | 0.0058 (3) | 0.0058 (3) | 0.0088 (3) | 0 | 0 | 0 |

$V_{0.8}Ti_{0.2}Al_3$

| Atom | U11 | U22 | U33 | U23 | U13 | U12 |
|---|---|---|---|---|---|---|
| V1 | 0.0047 (1) | 0.0047 (1) | 0.0050 (2) | 0 | 0 | 0 |
| Ti2 | 0.0047 (1) | 0.0047 (1) | 0.0050 (2) | 0 | 0 | 0 |
| Al3 | 0.0068 (2) | 0.0068 (2) | 0.0070 (2) | 0 | 0 | 0 |
| Al4 | 0.0067 (2) | 0.0067 (2) | 0.0089 (3) | 0 | 0 | 0 |

$VAl_3$

| Atom | U11 | U22 | U33 | U23 | U13 | U12 |
|---|---|---|---|---|---|---|
| V1 | 0.0057 (2) | 0.0057 (2) | 0.0030 (2) | 0 | 0 | 0 |
| Al2 | 0.0068 (2) | 0.0068 (2) | 0.0062 (3) | 0 | 0 | 0 |
| Al3 | 0.0065 (3) | 0.0065 (3) | 0.0081 (4) | 0 | 0 | 0 |
